# Supplementary material for: Developing Guidelines for Functionally-Grounded Evaluation of Explainable Artificial Intelligence using Tabular Data
Source: arXiv:2410.12803 ancillary file (2024-09-30)
Supplement: Supplementary file 1 [file slr_paper_supplementary_materials.pdf]

# Supplementary Materials: An Analysis of XAI Evaluation in Literature

March 2024

## 1 Fidelity to the Model

Table 1: The depth and extensiveness of works that evaluate explanation fidelity to the model.

| Criteria             | Category      | Setting                         | Papers                                                                |
|----------------------|---------------|---------------------------------|-----------------------------------------------------------------------|
| Internal Correctness | Paper Purpose | Domain-Based Evaluation         | [1, 2]                                                                |
|                      |               | General Purpose Evaluation      | [3, 4, 5, 6, 7]                                                       |
|                      |               | Open-Source Package Proposal    | [8]                                                                   |
|                      |               | Proposal of Evaluation Criteria | [9, 10]                                                               |
|                      |               | Task-Based Evaluation           | [11, 12, 13]                                                          |
|                      |               | XAI Method Extension Proposal   | [14, 15, 16, 17, 18, 19]                                              |
|                      |               | XAI Method Proposal             | [20, 21, 22, 23, 24, 25, 26]                                          |
|                      | Num. Datasets | 1                               | [21, 1, 2, 5, 8, 10, 14, 18, 22, 26]                                  |
|                      |               | 2 to 5                          | [3, 7, 11, 12, 13, 16, 19, 24, 25]                                    |
|                      |               | 6 to 10                         | [9, 20, 23]                                                           |
|                      |               | More than 10                    | [4, 15, 17, 6]                                                        |
|                      | Dataset Type  | Multivariate Time Series        | [1, 11, 19, 12, 2, 13]                                                |
|                      |               | Univariate Time Series          | [16]                                                                  |
|                      |               | Tabular                         | [9, 8, 3, 20, 4, 21, 15, 22, 16, 5, 17, 23, 24, 6, 18, 25, 7, 10, 26] |
|                      |               | Synthetic                       | [14, 20, 22, 5, 24]                                                   |

Table 1: The depth and extensiveness of works that evaluate explanation fidelity to the model.

| Criteria             | Category       | Setting                               | Papers                                                                                   |
|----------------------|----------------|---------------------------------------|------------------------------------------------------------------------------------------|
| Internal Correctness | Num. Models    | 1                                     | [8, 21, 23, 24, 18, 1, 2, 13]                                                            |
|                      |                | 2 to 5                                | [9, 14, 3, 20, 4, 15, 22, 5, 6, 25, 7, 11, 19, 12, 10, 26]                               |
|                      |                | 6 to 10                               | [16, 17]                                                                                 |
|                      | Model Types    | Kernel-Based                          | [14, 15, 25]                                                                             |
|                      |                | Linear-Based                          | [3, 20, 4, 22, 16, 5, 17, 25, 7, 26]                                                     |
|                      |                | Neural Network                        | [8, 3, 24, 1, 25, 11, 19, 12, 2, 10, 26]                                                 |
|                      |                | Probabilistic                         | [9]                                                                                      |
|                      |                | Rule-Based                            | [22, 5, 17]                                                                              |
|                      |                | Shapelet Classification               | [16]                                                                                     |
|                      |                | Tree-Based                            | [9, 14, 20, 4, 21, 15, 16, 17, 23, 6, 18, 25, 7, 11, 12, 13, 10]                         |
|                      | Num. XAI       | 1                                     | [21, 6, 19]                                                                              |
|                      |                | 2 to 5                                | [9, 14, 8, 20, 4, 15, 22, 16, 23, 24, 18, 1, 25, 7, 11, 12, 2, 13, 10, 26]               |
|                      |                | 6 to 10                               | [3, 5, 17]                                                                               |
|                      | XAI Types      | Feature Attribution                   | [14, 8, 3, 20, 4, 21, 15, 22, 16, 5, 23, 24, 6, 18, 1, 25, 7, 11, 19, 12, 2, 13, 10, 26] |
|                      |                | Rule-Based                            | [20, 5, 17]                                                                              |
|                      | XAI Techniques | LIME                                  | [9, 14, 8, 3, 20, 4, 22, 16, 5, 17, 23, 18, 1, 25, 7, 13, 10, 26]                        |
|                      |                | SHAP                                  | [9, 14, 8, 3, 4, 15, 22, 5, 17, 18, 1, 25, 7, 11, 12, 2, 13, 10]                         |
|                      |                | MAPLE                                 | [3, 5, 17, 18]                                                                           |
|                      |                | Anchor                                | [5, 17, 23]                                                                              |
|                      |                | Integrated Gradients                  | [3, 2]                                                                                   |
|                      |                | Complete Shapley Calculation          | [4, 15]                                                                                  |
|                      |                | BRL                                   | [5, 17]                                                                                  |
|                      |                | LORE                                  | [5, 17]                                                                                  |
|                      |                | Permutation Feature Importance        | [25, 12]                                                                                 |
|                      |                | LIME-SHAP Ensemble                    | [14]                                                                                     |
|                      |                | SmoothGrad                            | [3]                                                                                      |
|                      |                | APE                                   | [20]                                                                                     |
|                      |                | GSLs                                  | [20]                                                                                     |
|                      |                | Correlation-Based Shapley Calculation | [4]                                                                                      |

Table 1: The depth and extensiveness of works that evaluate explanation fidelity to the model.

| Criteria             | Category          | Setting                         | Papers                                              |
|----------------------|-------------------|---------------------------------|-----------------------------------------------------|
| Internal Correctness |                   | Coalition Formation Techniques  | [15]                                                |
|                      |                   | CIU                             | [22]                                                |
|                      |                   | S-LIME                          | [16]                                                |
|                      |                   | PALEX                           | [23]                                                |
|                      |                   | XAIR                            | [24]                                                |
|                      |                   | LRP                             | [24]                                                |
|                      |                   | IME                             | [18]                                                |
|                      |                   | SABAAS                          | [18]                                                |
|                      |                   | Altruist                        | [25]                                                |
|                      |                   | DALEX                           | [7]                                                 |
|                      |                   | Feature Omission                | [11]                                                |
|                      |                   | PALE                            | [21]                                                |
|                      |                   | CFC                             | [6]                                                 |
|                      |                   | TS-MULE                         | [19]                                                |
|                      |                   | LimeForTime                     | [2]                                                 |
|                      |                   | LMM                             | [26]                                                |
|                      |                   | LEMNA                           | [26]                                                |
|                      | Depth of Findings | Used for Other Criteria         | [3]                                                 |
|                      |                   | Observations Only               | [14, 22, 23, 24, 18, 7, 11, 19, 12, 13, 26]         |
|                      |                   | Consolidation of Findings       | [9, 4, 21, 15, 5, 17, 6, 1, 25, 2, 10]              |
|                      |                   | Cause Identification            | [20, 16]                                            |
| External Correctness | Paper Purpose     | Domain-Based Evaluation         | [27, 28, 29, 30]                                    |
|                      |                   | General Purpose Evaluation      | [7]                                                 |
|                      |                   | Open-Source Package Proposal    | [31]                                                |
|                      |                   | Proposal of Evaluation Criteria | [32]                                                |
|                      |                   | Single XAI Evaluation           | [33]                                                |
|                      |                   | Task-Based Evaluation           | [34]                                                |
|                      |                   | XAI Method Extension Proposal   | [16, 17, 35, 36, 37, 38]                            |
|                      |                   | XAI Method Proposal             | [39, 40, 20, 41, 42, 43, 44, 45, 46, 26]            |
|                      | Num. Datasets     | 1                               | [27, 28, 29, 35, 30, 36, 26]                        |
|                      |                   | 2 to 5                          | [39, 31, 34, 32, 41, 16, 42, 45, 37, 7, 33, 46, 38] |

Table 1: The depth and extensiveness of works that evaluate explanation fidelity to the model.

| Criteria             | Category            | Setting                 | Papers                                                                                          |
|----------------------|---------------------|-------------------------|-------------------------------------------------------------------------------------------------|
| External Correctness | Dataset Type        | 6 to 10                 | [40, 20, 43, 44]                                                                                |
|                      |                     | More than 10            | [17]                                                                                            |
|                      | Dataset Type        | Univariate Time Series  | [16]                                                                                            |
|                      |                     | Tabular                 | [39, 31, 34, 32, 40, 27, 28, 20, 41, 16, 29, 42, 17, 43, 35, 30, 44, 45, 37, 7, 33, 46, 38, 26] |
|                      |                     | Synthetic               | [36, 46]                                                                                        |
|                      | Num. Models         | 1                       | [39, 28, 29, 43, 35, 30, 44, 36, 37, 33, 38]                                                    |
|                      |                     | 2 to 5                  | [34, 32, 40, 27, 20, 41, 42, 45, 7, 46, 26]                                                     |
|                      |                     | 6 to 10                 | [31, 16, 17]                                                                                    |
|                      | Model Types         | Ensemble                | [34]                                                                                            |
|                      |                     | Kernel-Based            | [31, 40, 41, 42, 17, 45]                                                                        |
|                      |                     | Linear-Based            | [31, 32, 40, 27, 20, 16, 17, 7, 46, 26]                                                         |
|                      |                     | Neighbourhood-Based     | [31]                                                                                            |
|                      |                     | Neural Network          | [31, 32, 27, 41, 16, 42, 17, 45, 33, 46, 38, 26]                                                |
|                      |                     | Probabilistic           | [39]                                                                                            |
|                      |                     | Shapelet Classification | [16]                                                                                            |
|                      |                     | Tree-Based              | [39, 31, 34, 40, 27, 28, 20, 41, 16, 29, 42, 17, 43, 35, 30, 44, 36, 45, 37, 7, 46]             |
|                      | Num. XAI            | 1                       | [34, 33]                                                                                        |
|                      |                     | 2 to 5                  | [39, 31, 32, 40, 27, 28, 20, 41, 16, 29, 42, 43, 35, 30, 44, 36, 45, 37, 7, 46, 38, 26]         |
|                      |                     | 6 to 10                 | [17]                                                                                            |
|                      | XAI Types           | Feature Attribution     | [39, 31, 34, 32, 40, 27, 28, 20, 16, 29, 42, 35, 45, 7, 46, 38, 26]                             |
|                      |                     | Rule-Based              | [20, 41, 42, 17, 43, 30, 44, 45, 37, 7, 33]                                                     |
|                      |                     | Feature Profiling       | [36]                                                                                            |
|                      |                     | Feature Sets            | [45]                                                                                            |
|                      | XAI Techniques Used | LIME                    | [39, 31, 32, 40, 27, 28, 20, 16, 29, 42, 17, 35, 45, 7, 46, 38, 26]                             |
|                      |                     | SHAP                    | [31, 34, 32, 40, 27, 28, 29, 17, 7, 46]                                                         |
|                      |                     | Anchor                  | [41, 42, 17, 43, 44, 7, 33]                                                                     |

Table 1: The depth and extensiveness of works that evaluate explanation fidelity to the model.

| Criteria             | Category          | Setting                                    | Papers                                                                      |
|----------------------|-------------------|--------------------------------------------|-----------------------------------------------------------------------------|
| External Correctness |                   | LORE                                       | [42, 17, 30, 7]                                                             |
|                      |                   | AraucanaXAI                                | [27, 46]                                                                    |
|                      |                   | BRL                                        | [17, 43]                                                                    |
|                      |                   | CHIRPS                                     | [43, 44]                                                                    |
|                      |                   | LionForest                                 | [44, 37]                                                                    |
|                      |                   | defragTrees                                | [43, 44]                                                                    |
|                      |                   | ALIME                                      | [38]                                                                        |
|                      |                   | APE                                        | [20]                                                                        |
|                      |                   | C-LORE-F                                   | [30]                                                                        |
|                      |                   | CASTLE                                     | [41]                                                                        |
|                      |                   | CIE                                        | [45]                                                                        |
|                      |                   | Conditional PDP                            | [36]                                                                        |
|                      |                   | Conditional Permutation Feature Importance | [36]                                                                        |
|                      |                   | DALEX                                      | [7]                                                                         |
|                      |                   | DRSA                                       | [30]                                                                        |
|                      |                   | GSLs                                       | [20]                                                                        |
|                      |                   | LEMNA                                      | [26]                                                                        |
|                      |                   | LMM                                        | [26]                                                                        |
|                      |                   | MAPLE                                      | [17]                                                                        |
|                      |                   | Muse                                       | [45]                                                                        |
|                      |                   | PDP                                        | [36]                                                                        |
|                      |                   | Permutation Feature Importance             | [36]                                                                        |
|                      |                   | S-LIME                                     | [16]                                                                        |
|                      |                   | SLISE                                      | [40]                                                                        |
|                      |                   | Slisemap                                   | [40]                                                                        |
|                      |                   | Tree-LIME                                  | [35]                                                                        |
|                      |                   | inTrees                                    | [43]                                                                        |
|                      | Depth of Findings | Not Evaluated                              | [28]                                                                        |
|                      |                   | Used for Other Criteria                    | [32]                                                                        |
|                      |                   | Observations Only                          | [39, 31, 34, 40, 27, 29, 42, 17, 43, 35, 30, 44, 45, 37, 7, 33, 46, 38, 26] |
|                      |                   | Consolidation of Findings                  | [20, 36]                                                                    |
| Completeness         | Paper Purpose     | Cause Identification                       | [41, 16]                                                                    |
|                      |                   | Open-Source Package Proposal               | [8]                                                                         |
|                      |                   | Num. Datasets                              | [8]                                                                         |
|                      | Dataset Type      | Tabular                                    | [8]                                                                         |

Table 1: The depth and extensiveness of works that evaluate explanation fidelity to the model.

| Criteria             | Category          | Setting                         | Papers   |
|----------------------|-------------------|---------------------------------|----------|
| Completeness         | Num. Models       | 1                               | [8]      |
|                      | Model Types       | Neural Network                  | [8]      |
|                      | Num. XAI          | 2                               | [8]      |
|                      | XAI Types         | Feature Attribution             | [8]      |
|                      | XAI Techniques    | LIME                            | [8]      |
|                      | Used              | SHAP                            | [8]      |
| Necessity            | Depth of Findings | Observations Only               | [8]      |
|                      | Paper Purpose     | XAI Method Proposal             | [47]     |
|                      | Num. Datasets     | 1                               | [47]     |
|                      | Dataset Type      | Tabular                         | [47]     |
|                      | Num. Models       | 1                               | [47]     |
|                      | Model Types       | Tree-Based                      | [47]     |
|                      | Num. XAI          | 3                               | [47]     |
|                      | XAI Types         | Feature Attribution             | [47]     |
|                      |                   | Rule-Based                      | [47]     |
|                      | XAI Techniques    | LIME                            | [47]     |
|                      | Used              | SHAP                            | [47]     |
|                      |                   | LENS                            | [47]     |
| Sufficiency          | Depth of Findings | Not Evaluated                   | [47]     |
|                      | Paper Purpose     | XAI Method Proposal             | [44, 47] |
|                      | Num. Datasets     | 1                               | [47]     |
|                      |                   | 6 to 10                         | [44]     |
|                      | Dataset Type      | Tabular                         | [44, 47] |
|                      | Num. Models       | 1                               | [44, 47] |
|                      | Model Types       | Tree-Based                      | [44, 47] |
|                      | Num. XAI          | 2 to 5                          | [44, 47] |
|                      | XAI Types         | Rule-Based                      | [44, 47] |
|                      |                   | Feature Attribution             | [47]     |
|                      | XAI Techniques    | Anchor                          | [44]     |
|                      | Used              | CHIRPS                          | [44]     |
|                      |                   | defragTrees                     | [44]     |
|                      |                   | LionForest                      | [44]     |
|                      |                   | LIME                            | [47]     |
|                      |                   | SHAP                            | [47]     |
|                      |                   | LENS                            | [47]     |
|                      | Depth of Findings | Not Evaluated                   | [44]     |
|                      |                   | Not Evaluated                   | [47]     |
| Descriptive Accuracy | Paper Purpose     | Proposal of Evaluation Criteria | [9]      |

Table 1: The depth and extensiveness of works that evaluate explanation fidelity to the model.

| <b>Criteria</b>      | <b>Category</b>     | <b>Setting</b>      | <b>Papers</b> |
|----------------------|---------------------|---------------------|---------------|
| Descriptive Accuracy | Num. Datasets       | 7                   | [9]           |
|                      | Dataset Type        | Tabular             | [9]           |
|                      | Num. Models         | 4                   | [9]           |
|                      | Model Types         | Probabilistic       | [9]           |
|                      |                     | Tree-Based          | [9]           |
|                      | Num. XAI            | 2                   | [9]           |
|                      | XAI Types           | Feature Attribution | [9]           |
|                      | XAI Techniques Used | LIME                | [9]           |
|                      |                     | SHAP                | [9]           |
|                      | Depth of Findings   | Observations Only   | [9]           |

## 2 Explanation Invariance

Table 2: The depth and extensiveness of works that evaluate explanation invariance.

| Criteria                | Category      | Setting                       | Papers                                                                                                                                                                             |
|-------------------------|---------------|-------------------------------|------------------------------------------------------------------------------------------------------------------------------------------------------------------------------------|
| Explanation Sensitivity | Paper Purpose | Domain-Based Evaluation       | [48, 49, 50]                                                                                                                                                                       |
|                         |               | General Purpose Evaluation    | [3, 4, 51, 7]                                                                                                                                                                      |
|                         |               | Open-Source Package Proposal  | [8]                                                                                                                                                                                |
|                         |               | XAI Method Extension Proposal | [14, 52, 17]                                                                                                                                                                       |
|                         |               | XAI Method Proposal           | [53, 46]                                                                                                                                                                           |
|                         |               | Num. Datasets                 | 1 [53, 14, 52, 8, 48, 51, 49, 50]<br>2 to 5 [3, 7, 46]<br>More than 10 [4, 17]                                                                                                     |
|                         |               | Dataset Type                  | Multivariate Time Series [49]<br>Tabular [53, 14, 52, 8, 3, 4, 48, 17, 51, 7, 46, 50]<br>Synthetic [53, 14, 52, 46]                                                                |
| Num. Models             |               | 1                             | [52, 8, 48, 51]                                                                                                                                                                    |
|                         |               | 2 to 5                        | [53, 14, 3, 4, 49, 7, 46, 50]                                                                                                                                                      |
|                         |               | 6 to 10                       | [17]                                                                                                                                                                               |
|                         |               | Model Types                   | Ensemble [49]<br>Kernel-Based [53, 14, 17, 49, 50]<br>Linear-Based [3, 4, 17, 7, 46]<br>Neural Network [8, 3, 48, 17, 51, 49, 46, 50]<br>Tree-Based [53, 14, 52, 4, 17, 49, 7, 46] |
| Num. XAI                |               | 1                             | [52, 50]                                                                                                                                                                           |
|                         |               | 2 to 5                        | [53, 14, 8, 4, 48, 51, 49, 7, 46]                                                                                                                                                  |
|                         |               | 6 to 10                       | [3, 17]                                                                                                                                                                            |
| XAI Types               |               | Feature Attribution           | [53, 14, 52, 8, 3, 4, 48, 51, 49, 7, 46, 50]<br>Rule-Based [17, 7]                                                                                                                 |
|                         |               | XAI Techniques Used           | SHAP [53, 14, 8, 3, 4, 48, 17, 51, 49, 7, 46, 50]<br>LIME [53, 14, 8, 3, 4, 48, 17, 51, 49, 7, 46]<br>Anchor [17, 7]<br>LORE [17, 7]<br>MAPLE [3, 17]<br>AraucanaXAI [46]          |

Table 2: The depth and extensiveness of works that evaluate explanation fidelity to the model.

| Criteria                | Category          | Setting                                     | Papers                                                  |
|-------------------------|-------------------|---------------------------------------------|---------------------------------------------------------|
| Explanation Sensitivity |                   | BRL                                         | [17]                                                    |
|                         |                   | CIE                                         | [52]                                                    |
|                         |                   | Complete Shapley Value Calculation          | [4]                                                     |
|                         |                   | Correlation-Based Shapley Value Calculation | [4]                                                     |
|                         |                   | DALEX                                       | [7]                                                     |
|                         |                   | Integrated Gradients                        | [3]                                                     |
|                         |                   | LUX                                         | [53]                                                    |
|                         |                   | Model Coefficients                          | [52]                                                    |
|                         |                   | SHAP-LIME Ensemble                          | [14]                                                    |
|                         |                   | SmoothGrad                                  | [3]                                                     |
|                         |                   | VanillaGrad                                 | [3]                                                     |
|                         | Depth of Findings | Used for Other Criteria                     | [3]                                                     |
|                         |                   | Observations Only                           | [52, 8, 48, 17, 51, 7, 46, 50]                          |
|                         |                   | Consolidation of Findings                   | [53, 14, 4, 49]                                         |
| Explanation Similarity  | Paper Purpose     | Domain-Based Evaluation                     | [27, 28, 48]                                            |
|                         |                   | Domain-Specific XAI Proposal                | [54]                                                    |
|                         |                   | General Purpose Evaluation                  | [3, 51]                                                 |
|                         |                   | Open-Source Package Proposal                | [31]                                                    |
|                         |                   | Task-Based Evaluation                       | [55]                                                    |
|                         |                   | XAI Method Extension Proposal               | [17, 56, 38]                                            |
|                         |                   | XAI Method Proposal                         | [42, 44, 46, 57]                                        |
|                         | Num. Datasets     | 1                                           | [27, 28, 48, 51]                                        |
|                         |                   | 2 to 5                                      | [31, 3, 42, 54, 46, 56, 57, 38, 55]                     |
|                         |                   | 6 to 10                                     | [44]                                                    |
|                         |                   | More than 10                                | [17]                                                    |
|                         | Dataset Type      | Multivariate Time Series                    | [55]                                                    |
|                         |                   | Tabular                                     | [31, 27, 28, 3, 48, 42, 17, 51, 44, 54, 46, 56, 57, 38] |

Table 2: The depth and extensiveness of works that evaluate explanation fidelity to the model.

| Criteria               | Category            | Setting                 | Papers                                               |
|------------------------|---------------------|-------------------------|------------------------------------------------------|
| Explanation Similarity | Num. Models         | 1                       | [28, 48, 51, 44, 54, 56, 38]                         |
|                        |                     | 2 to 5                  | [27, 3, 42, 46, 57, 55]                              |
|                        |                     | 6 to 10                 | [31, 17]                                             |
|                        | Model Types         | Kernel-Based            | [31, 42, 17, 57]                                     |
|                        |                     | Linear-Based            | [31, 27, 3, 17, 46, 55]                              |
|                        |                     | Neighbourhood-Based     | [31]                                                 |
|                        |                     | Neural Network          | [31, 27, 3, 48, 42, 17, 51, 54, 46, 56, 38]          |
|                        |                     | Tree-Based              | [31, 27, 28, 42, 17, 44, 46, 57, 55]                 |
|                        | Num. XAI            | 2 to 5                  | [31, 27, 28, 48, 42, 51, 44, 54, 46, 56, 57, 38, 55] |
|                        |                     | 6 to 10                 | [3, 17]                                              |
|                        | XAI Types           | Feature Attribution     | [31, 27, 28, 3, 48, 42, 51, 54, 46, 56, 57, 38, 55]  |
|                        |                     | Rule-Based              | [42, 17, 44]                                         |
|                        | XAI Techniques Used | LIME                    | [31, 27, 28, 3, 48, 42, 17, 51, 46, 56, 57, 38, 55]  |
|                        |                     | SHAP                    | [31, 27, 28, 3, 48, 17, 51, 54, 46, 55]              |
|                        |                     | Anchor                  | [42, 17, 44]                                         |
|                        |                     | ALIME                   | [56, 38]                                             |
|                        |                     | AraucanaXAI             | [27, 46]                                             |
|                        |                     | LORE                    | [42, 17]                                             |
|                        |                     | MAPLE                   | [3, 17]                                              |
|                        |                     | ALIME-Tree              | [56]                                                 |
|                        |                     | APE                     | [54]                                                 |
|                        |                     | A-SHAP                  | [54]                                                 |
|                        |                     | BayLIME                 | [57]                                                 |
|                        |                     | BRL                     | [17]                                                 |
|                        |                     | CHIRPS                  | [44]                                                 |
|                        |                     | defragTrees             | [44]                                                 |
|                        |                     | Integrated Gradients    | [3]                                                  |
|                        |                     | LionForest              | [44]                                                 |
|                        |                     | RESHAPE                 | [54]                                                 |
|                        |                     | SmoothGrad              | [3]                                                  |
|                        |                     | Unravel                 | [57]                                                 |
|                        |                     | VanillaGrad             | [3]                                                  |
|                        | Depth of Findings   | Not Evaluated           | [27, 28]                                             |
|                        |                     | Used for Other Criteria | [3]                                                  |

Table 2: The depth and extensiveness of works that evaluate explanation fidelity to the model.

| Criteria                 |       | Category            | Setting                       | Papers               |
|--------------------------|-------|---------------------|-------------------------------|----------------------|
| Explanation Similarity   |       |                     | Observations Only             | [42, 17, 51, 44, 57] |
|                          |       |                     | Consolidation of Findings     | [46, 56]             |
|                          |       |                     | Cause Identification          | [31, 48, 38, 55]     |
| Explanation Separability | Sepa- | Paper Purpose       | Domain-Based Evaluation       | [27, 48]             |
|                          |       |                     | General Purpose Evaluation    | [51]                 |
|                          |       |                     | XAI Method Proposal           | [46]                 |
|                          |       |                     |                               |                      |
|                          |       | Num. Datasets       | 1                             | [27, 48, 51]         |
|                          |       |                     | 2 to 5                        | [46]                 |
|                          |       | Dataset Type        | Tabular                       | [27, 48, 51, 46]     |
|                          |       | Num. Models         | 1                             | [48, 51]             |
|                          |       |                     | 2 to 5                        | [27, 46]             |
|                          |       | Model Types         | Linear-Based                  | [27, 46]             |
|                          |       |                     | Neural Network                | [27, 48, 51, 46]     |
|                          |       |                     | Tree-Based                    | [27, 46]             |
|                          |       | Num. XAI            | 1                             | [27, 48, 51, 46]     |
|                          |       | XAI Types           | Feature Attribution           | [27, 48, 51, 46]     |
|                          |       | XAI Techniques Used | LIME                          | [27, 48, 51, 46]     |
|                          |       |                     | SHAP                          | [27, 48, 51, 46]     |
|                          |       |                     | AraucanaXAI                   | [27, 46]             |
|                          |       | Depth of Findings   | Observations Only             | [51]                 |
|                          |       |                     | Consolidation of Findings     | [27, 48, 46]         |
| Explanation Synonymity   | Syn-  | Paper Purpose       | Domain-Based Evaluation       | [49]                 |
|                          |       |                     | XAI Method Extension Proposal | [53]                 |
|                          |       |                     | XAI Method Proposal           | [53]                 |
|                          |       | Num. Datasets       | 1                             | [53, 14, 49]         |
|                          |       |                     |                               |                      |
|                          |       | Dataset Type        | Multivariate Time Series      | [49]                 |
|                          |       |                     | Tabular                       | [53, 14]             |
|                          |       |                     | Synthetic                     | [53, 14]             |
|                          |       | Num. Models         | 2 to 5                        | [53, 14, 49]         |
|                          |       | Model Types         | Ensemble                      | [49]                 |
|                          |       |                     | Kernel-Based                  | [53, 14, 49]         |
|                          |       |                     | Neural Network                | [49]                 |
|                          |       |                     | Tree-Based                    | [53, 14, 49]         |
|                          |       | Num. XAI            | 2 to 5                        | [53, 14, 49]         |

Table 2: The depth and extensiveness of works that evaluate explanation fidelity to the model.

| Criteria                  |      | Category               | Setting                   | Papers       |
|---------------------------|------|------------------------|---------------------------|--------------|
| Explanation<br>Synonymity | Syn- | XAI Types              | Feature Attribution       | [53, 14, 49] |
|                           |      | XAI Techniques<br>Used | LIME                      | [53, 14, 49] |
|                           |      |                        | SHAP                      | [53, 14, 49] |
|                           |      |                        | LUX                       | [53]         |
|                           |      |                        | SHAP-LIME Ensemble        | [14]         |
|                           |      | Depth of Findings      | Observations Only         | [14]         |
|                           |      |                        | Consolidation of Findings | [53, 49]     |

### 3 Fidelity to the Ground Truth

Table 3: The depth and extensiveness of works that evaluate explanation fidelity to the ground truth.

| Criteria    |               | Category            | Setting                       | Papers                               |
|-------------|---------------|---------------------|-------------------------------|--------------------------------------|
| Explanation | Cov-<br>erage | Paper Purpose       | XAI Method Extension Proposal | [58, 17, 37]                         |
|             |               |                     | XAI Method Proposal           | [40, 41, 42, 43, 44, 45]             |
|             |               | Num. Datasets       | 2 to 5                        | [58, 41, 42, 45, 37]                 |
|             |               |                     | 6 to 10                       | [40, 43, 44]                         |
|             |               |                     | More than 10                  | [17]                                 |
|             |               | Dataset Type        | Tabular                       | [40, 58, 41, 42, 17, 43, 44, 45, 37] |
|             |               | Num. Models         | 1                             | [43, 44, 37]                         |
|             |               |                     | 2 to 5                        | [40, 58, 41, 42, 45]                 |
|             |               |                     | 6 to 10                       | [17]                                 |
|             |               | Model Types         | Kernel-Based                  | [40, 58, 41, 42, 17, 45]             |
|             |               |                     | Linear-Based                  | [40, 58, 17]                         |
|             |               |                     | Neural Network                | [58, 41, 42, 17, 45]                 |
|             |               |                     | Tree-Based                    | [40, 58, 41, 42, 17, 43, 44, 45, 37] |
|             |               | Num. XAI            | 1                             | [45]                                 |
|             |               |                     | 2 to 5                        | [40, 58, 41, 42, 43, 44, 37]         |
|             |               |                     | 6 to 10                       | [17]                                 |
|             |               | XAI Types           | Feature Attribution           | [40]                                 |
|             |               |                     | Rule-Based                    | [58, 41, 42, 17, 43, 44, 45, 37]     |
|             |               | XAI Techniques Used | Anchor                        | [58, 41, 42, 17, 43, 44]             |
|             |               |                     | BRL                           | [17, 43]                             |
|             |               |                     | CHIRPS                        | [43, 44]                             |
|             |               |                     | defragTrees                   | [43, 44]                             |
|             |               |                     | LionForest                    | [44, 37]                             |
|             |               |                     | LORE                          | [42, 17]                             |
|             |               |                     | CASTLE                        | [41]                                 |
|             |               |                     | CIE                           | [45]                                 |
|             |               |                     | inTrees                       | [43]                                 |
|             |               |                     | LIME                          | [40]                                 |
|             |               |                     | SHAP                          | [40]                                 |
|             |               |                     | Slisemap                      | [40]                                 |
|             |               | Depth of Findings   | Not Evaluated                 | [45]                                 |
|             |               |                     | Observations Only             | [40, 58, 41, 42, 17, 43, 44, 37]     |
| Explanation | Real-<br>ism  | Paper Purpose       | Domain-Based Evaluation       | [59, 60, 50]                         |
|             |               |                     | Domain-Specific XAI Proposal  | [54]                                 |
|             |               |                     | General Purpose Evaluation    | [61]                                 |
|             |               |                     |                               |                                      |

Table 3: The depth and extensiveness of works that evaluate explanation fidelity to the model.

| Criteria            | Category            | Setting                            | Papers                   |
|---------------------|---------------------|------------------------------------|--------------------------|
| Explanation Realism |                     | XAI Method Proposal                | [23]                     |
|                     | Num. Datasets       | 1                                  | [23, 59, 50]             |
|                     |                     | 2 to 5                             | [54, 60]                 |
|                     |                     | 6 to 10                            | [61]                     |
|                     | Dataset Type        | Multivariate Time Series           | [60]                     |
|                     |                     | Tabular                            | [23, 59, 54, 61, 50]     |
|                     |                     | Synthetic                          | [61]                     |
|                     | Num. Models         | 1                                  | [54, 60, 61]             |
|                     |                     | 2 to 5                             | [23, 59, 50]             |
|                     | Model Types         | Kernel-Based                       | [50]                     |
|                     |                     | Linear-Based                       | [59]                     |
|                     |                     | Neural Network                     | [59, 54, 60, 61, 50]     |
|                     |                     | Synthetic                          | [23]                     |
|                     |                     | Tree-Based                         | [23, 59]                 |
|                     | Num. XAI            | 1                                  | [50]                     |
|                     |                     | 2 to 5                             | [23, 59, 54, 60]         |
|                     |                     | 6 to 10                            | [61]                     |
|                     | XAI Types           | Feature Attribution                | [23, 59, 54, 60, 61, 50] |
|                     |                     | Rule-Based                         | [59]                     |
|                     | XAI Techniques Used | SHAP                               | [59, 54, 60, 61, 50]     |
|                     |                     | LIME                               | [23, 59, 60, 61]         |
|                     |                     | Anchor                             | [23, 59]                 |
|                     |                     | Integrated Gradients               | [60, 61]                 |
|                     |                     | APE                                | [54]                     |
|                     |                     | A-SHAP                             | [54]                     |
|                     |                     | BEEF                               | [59]                     |
|                     |                     | Complete Shapley Value Calculation | [61]                     |
|                     |                     | DeepLIFT                           | [61]                     |
|                     |                     | e-LRP                              | [61]                     |
|                     |                     | GradientXInput                     | [61]                     |
|                     |                     | LORE                               | [59]                     |
|                     |                     | LRP                                | [61]                     |
|                     |                     | PALEX                              | [23]                     |
|                     |                     | RESHAPE                            | [54]                     |
|                     |                     | Saliency Map                       | [61]                     |
|                     | Depth of Findings   | Observations Only                  | [23, 54, 60, 50]         |
|                     |                     | Consolidation of Findings          | [59]                     |
|                     |                     | Cause Identification               | [61]                     |

Table 3: The depth and extensiveness of works that evaluate explanation fidelity to the model.

| Criteria                  | Category            | Setting                                    | Papers           |
|---------------------------|---------------------|--------------------------------------------|------------------|
| Realism of Synthetic Data | Paper Purpose       | XAI Method Extension Proposal              | [17, 36]         |
|                           |                     | XAI Method Proposal                        | [40, 57]         |
|                           | Num. Datasets       | 1                                          | [36]             |
|                           |                     | 2 to 5                                     | [57]             |
|                           |                     | 6 to 10                                    | [40]             |
|                           |                     | More than 10                               | [17]             |
|                           | Dataset Type        | Tabular                                    | [40, 17, 36, 57] |
|                           |                     | Synthetic                                  | [36]             |
|                           | Num. Models         | 2 to 5                                     | [40, 36, 57]     |
|                           |                     | 6 to 10                                    | [17]             |
|                           | Model Types         | Kernel-Based                               | [40, 17, 57]     |
|                           |                     | Linear-Based                               | [40, 17]         |
|                           |                     | Neural Network                             | [17]             |
|                           |                     | Synthetic                                  | [36]             |
|                           |                     | Tree-Based                                 | [40, 17, 36, 57] |
|                           | Num. XAI            | 2 to 5                                     | [40, 36, 57]     |
|                           |                     | 6 to 10                                    | [17]             |
|                           | XAI Types           | Feature Attribution                        | [40, 57]         |
|                           |                     | Rule-Based                                 | [17]             |
|                           |                     | Feature Profiling                          | [36]             |
|                           | XAI Techniques Used | LIME                                       | [40, 17, 57]     |
|                           |                     | SHAP                                       | [40, 17]         |
|                           |                     | Anchor                                     | [17]             |
|                           |                     | BayLIME                                    | [57]             |
|                           |                     | BRL                                        | [17]             |
|                           |                     | Conditional PDP                            | [36]             |
|                           |                     | Conditional Permutation Feature Importance | [36]             |
|                           |                     | LORE                                       | [17]             |
|                           |                     | MAPLE                                      | [17]             |
|                           |                     | PDP                                        | [36]             |
|                           |                     | Permutation Feature Importance             | [36]             |
|                           |                     | SLISE                                      | [40]             |
|                           |                     | Unravel                                    | [57]             |
|                           | Depth of Findings   | Observations Only                          | [40, 17, 36, 57] |

## 4 XAI Complexity

Table 4: The depth and extensiveness of works that evaluate XAI complexity.

| Criteria         | Category            | Setting                            | Papers                                             |
|------------------|---------------------|------------------------------------|----------------------------------------------------|
| Computation Time | Paper Purpose       | Domain-Based Evaluation            | [27, 28, 30, 2]                                    |
|                  |                     | General Purpose Evaluation         | [4]                                                |
|                  |                     | XAI Method Extension Proposal      | [15, 18, 37]                                       |
|                  |                     | XAI Method Proposal                | [40, 41, 43, 44, 46]                               |
|                  |                     |                                    |                                                    |
|                  | Num. Datasets       | 1                                  | [27, 28, 18, 30, 2]                                |
|                  |                     | 2 to 5                             | [41, 37, 46]                                       |
|                  |                     | 6 to 10                            | [40, 43, 44]                                       |
|                  |                     | More than 10                       | [4, 15]                                            |
|                  | Dataset Type        | Multivariate Time Series           | [2]                                                |
|                  |                     | Synthetic                          | [46]                                               |
|                  |                     | Tabular                            | [40, 27, 28, 4, 15, 41, 43, 18, 30, 44, 37, 46]    |
|                  | Num. Models         | 1                                  | [28, 43, 18, 30, 44, 37, 2]                        |
|                  |                     | 2 to 5                             | [40, 27, 4, 15, 41, 46]                            |
|                  | Model Types         | Kernel-Based                       | [40, 15, 41]                                       |
|                  |                     | Linear-Based                       | [40, 27, 4, 46]                                    |
|                  |                     | Neural Network                     | [27, 41, 46, 2]                                    |
|                  |                     | Tree-Based                         | [40, 27, 28, 4, 15, 41, 43, 18, 30, 44, 37, 46]    |
|                  | Num. XAI            | 2 to 5                             | [40, 27, 28, 4, 15, 41, 43, 18, 30, 44, 37, 46, 2] |
|                  | XAI Types           | Feature Attribution                | [40, 27, 28, 4, 15, 18, 46, 2]                     |
|                  |                     | Rule-Based                         | [41, 43, 30, 44, 37]                               |
|                  | XAI Techniques Used | SHAP                               | [40, 27, 28, 4, 15, 18, 46, 2]                     |
|                  |                     | LIME                               | [40, 27, 28, 4, 18, 46]                            |
|                  |                     | Anchor                             | [41, 43, 44]                                       |
|                  |                     | AraucanaXAI                        | [27, 46]                                           |
|                  |                     | CHIRPS                             | [43, 44]                                           |
|                  |                     | Complete Shapley Value Calculation | [4, 15]                                            |
|                  |                     | defragTrees                        | [43, 44]                                           |
|                  |                     | LionForest                         | [44, 37]                                           |
|                  |                     | BRL                                | [43]                                               |
|                  |                     | LORE                               | [30]                                               |

Table 4: The depth and extensiveness of works that evaluate XAI complexity.

| Criteria              | Category          | Setting                          | Papers                          |
|-----------------------|-------------------|----------------------------------|---------------------------------|
| Computation Time      |                   | MAPLE                            | [18]                            |
|                       |                   | SLISE                            | [40]                            |
|                       |                   | Slisemap                         | [40]                            |
|                       |                   | CASTLE                           | [41]                            |
|                       |                   | C-LORE-F                         | [30]                            |
|                       |                   | Coalition Formation Techniques   | [15]                            |
|                       |                   | Correlation-Based Shapley Values | [4]                             |
|                       |                   | DRSA                             | [30]                            |
|                       |                   | Integrated Gradients             | [2]                             |
|                       |                   | inTrees                          | [43]                            |
|                       |                   | SABAAS                           | [18]                            |
|                       | Depth of Findings | Observations Only                | [40, 27, 15, 41, 43, 18, 37, 2] |
|                       |                   | Consolidation of Findings        | [28, 4, 44, 46]                 |
|                       |                   | Cause Identification             | [30]                            |
| Explanation Parsimony | Paper Purpose     | Domain-Based Evaluation          | [1]                             |
|                       |                   | General Purpose Evaluation       | [3, 4]                          |
|                       |                   | Open-Source Package Proposal     | [31, 8]                         |
|                       |                   | Task-Based Evaluation            | [12]                            |
|                       |                   | XAI Method Extension Proposal    | [37]                            |
|                       |                   | XAI Method Proposal              | [44, 45]                        |
|                       | Num. Datasets     | 1                                | [8, 1]                          |
|                       |                   | 2 to 5                           | [31, 3, 45, 37, 12]             |
|                       |                   | 6 to 10                          | [44]                            |
|                       |                   | More than 10                     | [4]                             |
|                       | Dataset Type      | Multivariate Time Series         | [1, 12]                         |
|                       |                   | Tabular                          | [31, 8, 3, 4, 44, 45, 37]       |
|                       | Num. Models       | 1                                | [8, 1, 44, 37]                  |
|                       |                   | 2 to 5                           | [3, 4, 45, 12]                  |
|                       |                   | 6 to 10                          | [31]                            |
|                       | Model Types       | Kernel-Based                     | [31, 45]                        |
|                       |                   | Linear-Based                     | [31, 3, 4]                      |

Table 4: The depth and extensiveness of works that evaluate XAI complexity.

| Criteria              | Category            | Setting                            | Papers                  |
|-----------------------|---------------------|------------------------------------|-------------------------|
| Explanation Parsimony |                     | Neighbourhood-Based                | [31]                    |
|                       |                     | Neural Network                     | [31, 8, 3, 1, 45, 12]   |
|                       |                     | Tree-Based                         | [31, 4, 44, 45, 37, 12] |
|                       | Num. XAI            | 1                                  | [45, 37]                |
|                       |                     | 2 to 5                             | [31, 8, 4, 1, 44, 12]   |
|                       |                     | 6 to 10                            | [3]                     |
|                       | XAI Types           | Feature Attribution                | [31, 8, 3, 4, 1, 12]    |
|                       |                     | Rule-Based                         | [44, 45, 37]            |
|                       | XAI Techniques Used | LIME                               | [31, 8, 3, 4, 1]        |
|                       |                     | SHAP                               | [31, 8, 3, 4, 1, 12]    |
|                       |                     | LionForest                         | [44, 37]                |
|                       |                     | Anchor                             | [44]                    |
|                       |                     | MAPLE                              | [3]                     |
|                       |                     | CHIRPS                             | [44]                    |
|                       |                     | CIE                                | [45]                    |
|                       |                     | Complete Shapley Value Calculation | [4]                     |
|                       |                     | defragTrees                        | [44]                    |
|                       |                     | Integrated Gradients               | [3]                     |
|                       |                     | Permutation Feature Importance     | [12]                    |
|                       |                     | SmoothGrad                         | [3]                     |
|                       |                     | VanillaGrad                        | [3]                     |
|                       | Depth of Findings   | Not Evaluated                      | [31]                    |
|                       |                     | Used for Other Criteria            | [3, 45]                 |
|                       |                     | Observations Only                  | [8, 44, 37, 12]         |
|                       |                     | Consolidation of Findings          | [4]                     |
|                       |                     | Cause Identification               | [1]                     |

## 5 Explanation Safety

Table 5: The depth and extensiveness of works that evaluate explanation safety.

| Criteria               | Category            | Setting                       | Papers  |
|------------------------|---------------------|-------------------------------|---------|
| Subgroup Fairness      | Paper Purpose       | General Purpose Evaluation    | [3]     |
|                        |                     | XAI Method Extension Proposal | [32]    |
|                        | Num. Datasets       | 2 to 5                        | [32, 3] |
|                        | Dataset Type        | Tabular                       | [32, 3] |
|                        | Num. Models         | 2 to 5                        | [32, 3] |
|                        | Model Types         | Linear-Based                  | [32, 3] |
|                        |                     | Neural Network                | [32, 3] |
|                        | Num. XAI            | 2 to 5                        | [32]    |
|                        |                     | 6 to 10                       | [3]     |
|                        | XAI Types           | Feature Attribution           | [32, 3] |
|                        | XAI Techniques Used | LIME                          | [32, 3] |
|                        |                     | SHAP                          | [32, 3] |
|                        |                     | Integrated Gradients          | [3]     |
|                        |                     | MAPLE                         | [3]     |
|                        |                     | SmoothGrad                    | [3]     |
|                        |                     | VanillaGrad                   | [3]     |
|                        | Depth of Findings   | Consolidation of Findings     | [32, 3] |
| Adversarial Robustness | Paper Purpose       | XAI Method Extension Proposal | [62]    |
|                        |                     |                               |         |
|                        | Num. Datasets       | 2 to 5                        | [62]    |
|                        | Dataset Type        | Tabular                       | [62]    |
|                        | Num. Models         | 2 to 5                        | [62]    |
|                        | Model Types         | Kernel-Based                  | [62]    |
|                        |                     | Neural Network                | [62]    |
|                        |                     | Probabilistic                 | [62]    |
|                        |                     | Tree-Based                    | [62]    |
|                        | Num. XAI            | 6 to 10                       | [62]    |
|                        | XAI Types           | Feature Attribution           | [62]    |
|                        | XAI Techniques Used | LIME                          | [62]    |
|                        |                     | SHAP                          | [62]    |
|                        |                     | IME                           | [62]    |
|                        |                     | gLIME                         | [62]    |
|                        |                     | gSHAP                         | [62]    |
|                        |                     | gIME                          | [62]    |
|                        | Depth of Findings   | Cause Identification          | [62]    |

## 6 Application Utility

Table 6: The depth and extensiveness of works that evaluate application utility.

| Criteria                 | Category            | Setting                            | Papers   |
|--------------------------|---------------------|------------------------------------|----------|
| Task Suitability         | Paper Purpose       | Domain-Based Evaluation            | [63]     |
|                          |                     | Task-Based Evaluation              | [64]     |
|                          | Num. Datasets       | 1                                  | [63, 64] |
|                          | Dataset Type        | Multivariate Time Series           | [63]     |
|                          |                     | Tabular                            | [64]     |
|                          | Num. Models         | 1                                  | [64]     |
|                          |                     | 2 to 5                             | [63]     |
|                          | Model Types         | Linear-Based                       | [63]     |
|                          |                     | Neural Network                     | [63, 64] |
|                          | Num. XAI            | 1                                  | [63]     |
|                          |                     | 2 to 5                             | [64]     |
|                          | XAI Types           | Feature Attribution                | [63, 64] |
|                          | XAI Techniques Used | SHAP                               | [63, 64] |
|                          |                     | LIME                               | [64]     |
|                          |                     | Complete Shapley Value Calculation | [64]     |
|                          | Depth of Findings   | Observations Only                  | [63, 64] |
| Prediction Appraisal     | Paper Purpose       | Task-Based Evaluation              | [34]     |
|                          |                     |                                    |          |
|                          | Num. Datasets       | 2 to 5                             | [34]     |
|                          | Dataset Type        | Tabular                            | [34]     |
|                          | Num. Models         | 2 to 5                             | [34]     |
|                          |                     |                                    |          |
|                          | Model Types         | Ensemble                           | [34]     |
|                          |                     | Tree-Based                         | [34]     |
|                          | Num. XAI            | 1                                  | [34]     |
|                          | XAI Types           | Feature Attribution                | [34]     |
| Degree of Explainability | XAI Techniques Used | SHAP                               | [34]     |
|                          |                     |                                    |          |
|                          | Depth of Findings   | Observations Only                  | [34]     |
|                          | Paper Purpose       | Proposal of Evaluation Criteria    | [65]     |
|                          |                     |                                    |          |
|                          | Num. Datasets       | 1                                  | [65]     |
|                          | Dataset Type        | Tabular                            | [65]     |
|                          | Num. Models         | 1                                  | [65]     |
|                          |                     |                                    |          |
|                          | Model Types         | Tree-Based                         | [65]     |
|                          |                     |                                    |          |
|                          | Num. XAI            | 1                                  | [65]     |

Table 6: The depth and extensiveness of works that evaluate application utility.

| Criteria                 | Category          |            | Setting             | Papers |
|--------------------------|-------------------|------------|---------------------|--------|
| Degree of Explainability | XAI Types         |            | Feature Attribution | [65]   |
|                          | XAI Used          | Techniques | SHAP                | [65]   |
|                          | Depth of Findings |            | Observations Only   | [65]   |

## References

- [1] N. Maltbie, N. Niu, M. V. Doren, R. Johnson, XAI tools in the public sector: a case study on predicting combined sewer overflows, in: Proceedings of the 29th ACM Joint Meeting on European Software Engineering Conference and Symposium on the Foundations of Software Engineering, ACM, 2021. doi:10.1145/3468264.3468547.
- [2] M. Veerappa, M. Anneken, N. Burkart, M. F. Huber, Validation of XAI explanations for multivariate time series classification in the maritime domain, Journal of Computational Science 58 (2022) 101539. doi:10.1016/j.jocs.2021.101539.
- [3] J. Dai, S. Upadhyay, U. Aivodji, S. H. Bach, H. Lakkaraju, Fairness via explanation quality, in: Proceedings of the 2022 AAAI/ACM Conference on AI, Ethics, and Society, ACM, 2022. doi:10.1145/3514094.3534159.
- [4] E. Doumard, J. Aligon, E. Escriva, J.-B. Excoffier, P. Monsarrat, C. Soulé-Dupuy, A quantitative approach for the comparison of additive local explanation methods, Information Systems 114 (2023) 102162. doi:10.1016/j.is.2022.102162.
- [5] R. Guidotti, Evaluating local explanation methods on ground truth, Artificial Intelligence 291 (2021) 103428. doi:10.1016/j.artint.2020.103428.
- [6] M. Loecher, D. Lai, W. Qi, Approximation of SHAP values for randomized tree ensembles, in: Lecture Notes in Computer Science, Springer International Publishing, 2022, pp. 19–30. doi:10.1007/978-3-031-14463-9\_2.
- [7] F. Naretto, F. Bodria, F. Giannotti, D. Pedreschi, Benchmark analysis of black-box local explanation methods, in: The Third Italian Workshop on Explainable Artificial Intelligence, co-located with the 21st International Conference of the Italian Association for Artificial intelligence, 2022.  
URL <https://ceur-ws.org/Vol-3277/paper5.pdf>
- [8] R. Cugny, J. Aligon, M. Chevalier, G. R. Jimenez, O. Teste, AutoXAI, in: Proceedings of the 31st ACM International Conference on Information & Knowledge Management, ACM, 2022. doi:10.1145/3511808.3557247.
- [9] E. Albini, A. Rago, P. Baroni, F. Toni, Descriptive accuracy in explanations: The case of probabilistic classifiers, in: Lecture Notes in Computer Science, Springer International Publishing, 2022, pp. 279–294. doi:10.1007/978-3-031-18843-5\_19.

- [10] Y. Zhang, F. Xu, J. Zou, O. L. Petrosian, K. V. Krinkin, XAI evaluation: Evaluating black-box model explanations for prediction, in: 2021 II International Conference on Neural Networks and Neurotechnologies (NeuroNT), IEEE, 2021. doi:10.1109/neuront53022.2021.9472817.
- [11] O. Ozyegen, I. Ilic, M. Cevik, Evaluation of interpretability methods for multivariate time series forecasting, *Applied Intelligence* 52 (5) (2021) 4727–4743. doi:10.1007/s10489-021-02662-2.
- [12] A. Stevens, J. D. Smedt, J. Peepkorn, Quantifying explainability in outcome-oriented predictive process monitoring, in: *Lecture Notes in Business Information Processing*, Springer International Publishing, 2022, pp. 194–206. doi:10.1007/978-3-030-98581-3\_15.
- [13] M. Velmurugan, C. Ouyang, C. Moreira, R. Sindhgatta, Evaluating fidelity of explainable methods for predictive process analytics, in: *CAiSE Forum 2021: Intelligent Information Systems*, Springer International Publishing, 2021, pp. 64–72. doi:10.1007/978-3-030-79108-7\_8.
- [14] S. Bobek, P. Bałaga, G. J. Nalepa, Towards model-agnostic ensemble explanations, in: *Computational Science – ICCS 2021*, Springer International Publishing, 2021, pp. 39–51. doi:10.1007/978-3-030-77970-2\_4.
- [15] G. Ferrettini, E. Escriva, J. Aligon, J.-B. Excoffier, C. Soulé-Dupuy, Coalitional strategies for efficient individual prediction explanation, *Information Systems Frontiers* 24 (1) (2021) 49–75. doi:10.1007/s10796-021-10141-9.
- [16] R. Gaudel, L. Galárraga, J. Delaunay, L. Rozé, V. Bhargava, s-LIME: Reconciling locality and fidelity in linear explanations, in: *Lecture Notes in Computer Science*, Springer International Publishing, 2022, pp. 102–114. doi:10.1007/978-3-031-01333-1\_9.
- [17] R. Guidotti, A. Monreale, S. Ruggieri, F. Naretto, F. Turini, D. Pedreschi, F. Giannotti, Stable and actionable explanations of black-box models through factual and counterfactual rules, *Data Mining and Knowledge Discovery* (nov 2022). doi:10.1007/s10618-022-00878-5.
- [18] S. M. Lundberg, G. Erion, H. Chen, A. DeGrave, J. M. Prutkin, B. Nair, R. Katz, J. Himmelfarb, N. Bansal, S.-I. Lee, From local explanations to global understanding with explainable AI for trees, *Nature Machine Intelligence* 2 (1) (2020) 56–67. doi:10.1038/s42256-019-0138-9.
- [19] U. Schlegel, D. L. Vo, D. A. Keim, D. Seebacher, TS-MULE: Local interpretable model-agnostic explanations for time series forecast models, in: *Communications in Computer and Information Science*, Springer International Publishing, 2021, pp. 5–14. doi:10.1007/978-3-030-93736-2\_1.
- [20] J. Delaunay, L. Galárraga, C. Largouët, When should we use linear explanations?, in: *Proceedings of the 31st ACM International Conference on Information & Knowledge Management*, ACM, 2022. doi:10.1145/3511808.3557489.
- [21] J. Duell, X. Fan, M. Seisenberger, Towards polynomial adaptive local explanations for healthcare classifiers, in: *Lecture Notes in Computer Science*, Springer International Publishing, 2022, pp. 411–420. doi:10.1007/978-3-031-16564-1\_39.
- [22] K. Främling, Contextual importance and utility: A theoretical foundation, in: *Lecture Notes in Computer Science*, Springer International Publishing, 2022, pp. 117–128. doi:10.1007/978-3-030-97546-3\_10.

- [23] Y. Jia, J. Bailey, K. Ramamohanarao, C. Leckie, X. Ma, Exploiting patterns to explain individual predictions, *Knowledge and Information Systems* 62 (3) (2019) 927–950. doi:10.1007/s10115-019-01368-9.
- [24] S. Letzgus, P. Wagner, J. Lederer, W. Samek, K.-R. Muller, G. Montavon, Toward explainable artificial intelligence for regression models: A methodological perspective, *IEEE Signal Processing Magazine* 39 (4) (2022) 40–58. doi:10.1109/msp.2022.3153277.
- [25] I. Mollas, N. Bassiliades, G. Tsoumakas, Altruist: Argumentative explanations through local interpretations of predictive models, in: *Proceedings of the 12th Hellenic Conference on Artificial Intelligence*, ACM, 2022. doi:10.1145/3549737.3549762.
- [26] Z. Zhou, M. Sun, J. Chen, A Model-Agnostic Approach for Explaining the Predictions on Clustered Data, in: *2019 IEEE International Conference on Data Mining (ICDM)*, IEEE, 2019. doi:10.1109/icdm.2019.00202.
- [27] T. M. Buonocore, G. Nicora, A. Dagliati, E. Parimbelli, Evaluation of XAI on ALS 6-months mortality prediction, in: *Proceedings of the Working Notes of CLEF 2022 - Conference and Labs of the Evaluation Forum*, 2022.  
URL <https://ceur-ws.org/Vol-3180/paper-90.pdf>
- [28] Y. Chen, D. M. Aleman, T. G. Purdie, C. McIntosh, Understanding machine learning classifier decisions in automated radiotherapy quality assurance, *Physics in Medicine & Biology* 67 (2) (2022) 025001. doi:10.1088/1361-6560/ac3e0e.
- [29] A. Gramegna, P. Giudici, SHAP and LIME: An evaluation of discriminative power in credit risk, *Frontiers in Artificial Intelligence* 4 (sep 2021). doi:10.3389/frai.2021.752558.
- [30] N. Maaroo, A. Moreno, A. Valls, M. Jabreel, M. Szelag, A comparative study of two rule-based explanation methods for diabetic retinopathy risk assessment, *Applied Sciences* 12 (7) (2022) 3358. doi:10.3390/app12073358.
- [31] E. Amparore, A. Perotti, P. Bajardi, To trust or not to trust an explanation: using LEAF to evaluate local linear XAI methods, *PeerJ Computer Science* 7 (2021) e479. doi:10.7717/peerj-cs.479.
- [32] A. Balagopalan, H. Zhang, K. Hamidieh, T. Hartvigsen, F. Rudzicz, M. Ghassemi, The road to explainability is paved with bias: Measuring the fairness of explanations, in: *2022 ACM Conference on Fairness, Accountability, and Transparency*, ACM, 2022. doi:10.1145/3531146.3533179.
- [33] N. Narodytska, A. Shrotri, K. S. Meel, A. Ignatiev, J. Marques-Silva, Assessing heuristic machine learning explanations with model counting, in: *Lecture Notes in Computer Science*, Springer International Publishing, 2019, pp. 267–278. doi:10.1007/978-3-030-24258-9\_19.
- [34] Y. Arslan, B. Lebigot, K. Allix, L. Veiber, C. Lefebvre, A. Boytsov, A. Goujon, T. Bissyande, J. Klein, On the suitability of SHAP explanations for refining classifications, in: *Proceedings of the 14th International Conference on Agents and Artificial Intelligence*, SCITEPRESS - Science and Technology Publications, 2022. doi:10.5220/0010827700003116.
- [35] H. Li, W. Fan, S. Shi, Q. Chou, A modified LIME and its application to explain service supply chain forecasting, in: *Natural Language Processing and Chinese Computing*, Springer International Publishing, 2019, pp. 637–644. doi:10.1007/978-3-030-32236-6\_58.

- [36] C. Molnar, G. König, B. Bischl, G. Casalicchio, Model-agnostic feature importance and effects with dependent features: a conditional subgroup approach, *Data Mining and Knowledge Discovery* (jan 2023). doi:10.1007/s10618-022-00901-9.
- [37] N. Mylonas, I. Mollas, N. Bassiliades, G. Tsoumakas, Local Multi-label Explanations for Random Forest, in: *Communications in Computer and Information Science*, Springer Nature Switzerland, 2023, pp. 369–384. doi:10.1007/978-3-031-23618-1\_25.
- [38] S. M. Shankaranarayana, D. Runje, ALIME: Autoencoder Based Approach for Local Interpretability, in: *Intelligent Data Engineering and Automated Learning – IDEAL*, 2019. doi:10.1007/978-3-030-33607-3\_49.
- [39] H. Afrabandpey, T. Peltola, J. Piironen, A. Vehtari, S. Kaski, A decision-theoretic approach for model interpretability in bayesian framework, *Machine Learning* 109 (9-10) (2020) 1855–1876. doi:10.1007/s10994-020-05901-8.
- [40] A. Björklund, J. Mäkelä, K. Puolamäki, SLISEMAP: supervised dimensionality reduction through local explanations, *Machine Learning* 112 (1) (2022) 1–43. doi:10.1007/s10994-022-06261-1.
- [41] V. La Gatta, V. Moscato, M. Postiglione, G. Sperli, CASTLE: Cluster-aided space transformation for local explanations, *Expert Systems with Applications* 179 (2021) 115045. doi:10.1016/j.eswa.2021.115045.
- [42] R. Guidotti, A. Monreale, F. Giannotti, D. Pedreschi, S. Ruggieri, F. Turini, Factual and Counterfactual Explanations for Black Box Decision Making, *IEEE Intelligent Systems* 34 (6) (2019) 14–23. doi:10.1109/mis.2019.2957223.
- [43] J. Hatwell, M. M. Gaber, R. M. A. Azad, CHIRPS: Explaining random forest classification, *Artificial Intelligence Review* 53 (8) (2020) 5747–5788. doi:10.1007/s10462-020-09833-6.
- [44] I. Mollas, N. Bassiliades, G. Tsoumakas, Conclusive local interpretation rules for random forests, *Data Mining and Knowledge Discovery* 36 (4) (2022) 1521–1574. doi:10.1007/s10618-022-00839-y.
- [45] M. Moradi, M. Samwald, Post-hoc explanation of black-box classifiers using confident itemsets, *Expert Systems with Applications* 165 (2021) 113941. doi:10.1016/j.eswa.2020.113941.
- [46] E. Parimbelli, T. M. Buonocore, G. Nicora, W. Michalowski, S. Wilk, R. Bellazzi, Why did AI get this one wrong? — tree-based explanations of machine learning model predictions, *Artificial Intelligence in Medicine* 135 (2023) 102471. doi:10.1016/j.artmed.2022.102471.
- [47] D. S. Watson, L. Gultchin, A. Taly, L. Floridi, Local explanations via necessity and sufficiency: Unifying theory and practice, *Minds and Machines* 32 (1) (2022) 185–218. doi:10.1007/s11023-022-09598-7.
- [48] A. Ferraro, A. Galli, V. Moscato, G. Sperli, Evaluating eXplainable artificial intelligence tools for hard disk drive predictive maintenance, *Artificial Intelligence Review* 56 (7) (2022) 7279–7314. doi:10.1007/s10462-022-10354-7.
- [49] J. Jakubowski, P. Stanis, S. Bobek, G. J. Nalepa, Performance of explainable AI methods in asset failure prediction, in: *Computational Science – ICCS 2022*, Springer International Publishing, 2022, pp. 472–485. doi:10.1007/978-3-031-08760-8\_40.

- [50] J. Tritscher, D. Schlör, F. Gwinner, A. Krause, A. Hotho, Towards explainable occupational fraud detection, in: *Communications in Computer and Information Science*, Springer Nature Switzerland, 2023, pp. 79–96. doi:10.1007/978-3-031-23633-4\_7.
- [51] Y. Hailemariam, A. Yazdinejad, R. M. Parizi, G. Srivastava, A. Dehghantanha, An Empirical Evaluation of AI Deep Explainable Tools, in: *2020 IEEE Globecom Workshops (GC Wkshps)*, IEEE, 2020. doi:10.1109/gewkshps50303.2020.9367541.
- [52] T. Botari, R. Izbicki, A. C. P. L. F. de Carvalho, Local interpretation methods to machine learning using the domain of the feature space, in: *Machine Learning and Knowledge Discovery in Databases*, Springer International Publishing, 2020, pp. 241–252. doi:10.1007/978-3-030-43823-4\_21.
- [53] S. Bobek, G. J. Nalepa, Introducing uncertainty into explainable AI methods, in: *Computational Science – ICCS 2021*, Springer International Publishing, 2021, pp. 444–457. doi:10.1007/978-3-030-77980-1\_34.
- [54] R. Müller, M. Schreyer, T. Sattarov, D. Borth, RESHAPE: Explaining accounting anomalies in financial statement audits by enhancing SHapley additive exPlanations, in: *Proceedings of the Third ACM International Conference on AI in Finance*, ACM, 2022. doi:10.1145/3533271.3561667.
- [55] M. Velmurugan, C. Ouyang, C. Moreira, R. Sindhgatta, Evaluating Stability of Post-hoc Explanations for Business Process Predictions, in: *ICSOC2021: Service-Oriented Computing*, 2021. doi:10.1007/978-3-030-91431-8\_4.
- [56] N. Ranjbar, R. Safabakhsh, Using decision tree as local interpretable model in autoencoder-based LIME, in: *2022 27th International Computer Conference, Computer Society of Iran (CSICC)*, IEEE, 2022. doi:10.1109/csicc55295.2022.9780503.
- [57] A. Saini, R. Prasad, Select wisely and explain: Active learning and probabilistic local post-hoc explainability, in: *Proceedings of the 2022 AAAI/ACM Conference on AI, Ethics, and Society*, ACM, 2022. doi:10.1145/3514094.3534191.
- [58] J. Delaunay, L. Galárraga, C. Largouët, Improving Anchor-based Explanations, in: *Proceedings of the 29th ACM International Conference on Information & Knowledge Management*, ACM, 2020. doi:10.1145/3340531.3417461.
- [59] V. Moscato, A. Picariello, G. Sperli, A benchmark of machine learning approaches for credit score prediction, *Expert Systems with Applications* 165 (2021) 113986. doi:10.1016/j.eswa.2020.113986.
- [60] J. Sipple, A. Youssef, A general-purpose method for applying explainable AI for anomaly detection, in: *Lecture Notes in Computer Science*, Springer International Publishing, 2022, pp. 162–174. doi:10.1007/978-3-031-16564-1\_16.
- [61] J. Tritscher, M. Ring, D. Schlr, L. Hettinger, A. Hotho, Evaluation of post-hoc XAI approaches through synthetic tabular data, in: *Lecture Notes in Computer Science*, Springer International Publishing, 2020, pp. 422–430. doi:10.1007/978-3-030-59491-6\_40.
- [62] D. Vreš, M. Robnik-Šikonja, Preventing deception with explanation methods using focused sampling, *Data Mining and Knowledge Discovery* (dec 2022). doi:10.1007/s10618-022-00900-w.

- [63] M. L. Baptista, K. Goebel, E. M. Henriques, Relation between prognostics predictor evaluation metrics and local interpretability SHAP values, *Artificial Intelligence* 306 (2022) 103667. doi:10.1016/j.artint.2022.103667.
- [64] E. Melo, I. Silva, D. G. Costa, C. M. D. Viegas, T. M. Barros, On the use of eXplainable artificial intelligence to evaluate school dropout, *Education Sciences* 12 (12) (2022) 845. doi:10.3390/educsci12120845.
- [65] F. Sovrano, F. Vitali, How to quantify the degree of explainability: Experiments and practical implications, in: 2022 IEEE International Conference on Fuzzy Systems (FUZZ-IEEE), IEEE, 2022. doi:10.1109/fuzz-ieee55066.2022.9882574.
